# Supplementary material for: Global Rewards in Restless Multi-Armed Bandits
Source: arXiv:2406.00738 source file (2024-06-07)
Supplement: Supplementary file 1 [file appendix.tex]

\section{Algorithm Details}
\begin{algorithm}[H]
\SetAlgoLined
\KwResult{Pull agents based on Q values}
Let $Q_0$ be 0 for all values\;
Let $V$ be 0 for all values\;
Let $i=0$\;
Let $\mathcal{S}=\{0,1\}$

\While {$i=0$ or $||Q_i-Q_{i-1}|| \geq \delta$}{

\For{each state combination $\{ s_{1} \ldots s_{N}\} \in \mathcal{S}^{N}$}
{
    \For{each set of actions $\{a_{1} \cdots a_{N}\}, \sum_{i=1}^{N} a_{i} = K$}{
        $Q_{i}(\{ s_{1} \ldots s_{N} \},\{a_{1} \cdots a_{N} \}) = -(1-p)^{\sum_{i=1}^{N} a_{i} \mathbbm{1}[s_{i} \in E]}$ \\
    $+ \gamma \sum_{\{ s_{1}^{'} \ldots s_{N}^{'} \}}$ 
    $\mathbb{P}(\{ s_{1} \ldots s_{N} \} \rightarrow \{ s_{1}^{'} \ldots s_{N}^{'} \} | a) V(\{ s_{1}^{'} \ldots s_{N}^{'}\}) $; \\  
    $V(\{ s_{1} \ldots s_{N}\})  = \mathrm{max}_{a} Q(\{ s_{1} \ldots s_{N}\},a)$ \;
    Increment $i$
        }
    }

}

Given a set of arms $\{s_{1} \ldots s_{N}\}$, play the action corresponding to $\mathrm{argmax}_a Q(\{s_{1} \ldots s_{N}\},a)$

 \caption{Q-Iteration for Matching}
\end{algorithm}

\begin{algorithm}[H]
\SetAlgoLined
\KwResult{Pull Agents by Solving Bilinear Optimization}
Consider $N$ agents to be in state $s_{i}^{t}$\; 
Consider the optimization problem $\sum_{i=1}^{N} a_{i}^{t} s_{i}^{t}$

\For{each agent $i$}{
    Let $w_i$ be the Whittle index\; 
    \While{Binary Search is not completed}{
        Let $m_i$ be the current estimation for the Whittle index \;
        Perform Q-iteration with the following update: 
        \begin{equation}
            Q(s_{i}^{t},a_{i}^{t} = -m_i*a_{i}^{t} + a_{i}^{t}*s_{i}^{t} + \gamma \sum_{s_{i}^{t+1}} P(s_{i}^{t+1} | s_{i}^{t}, a_{i}^{t})*V(s_{i}^{t+1})
        \end{equation}
        Compute the $Q$ values for $Q^{m_i}(s_{i}^{t},0)$, $Q^{m_i}(s_{i}^{t},1)$ \; 
        
        If $Q^{m_i}(s_{i}^{t},0) > Q^{m_i}(s_{i}^{t},1)$, then decrease $m_i$\;
        Otherwise, increase $m_i$
    }
    Let $w_i$ be the resulting value for $m_i$
}
Pick the arms with the $K$ highest values for $w_i$

 \caption{Whittle-Index for Matching}
\end{algorithm}

\begin{algorithm}[H]
\SetAlgoLined
\KwResult{Pull Agents by Solving Sufficient Q Iteration}
Consider $N$ agents to be in state $s_{i}^{t}$\; 
Let $T_{i}^{t} = \sum_{i=1}^{N} s_{i}^{t}$\;
Let $P(T^{t} = k) = P(\mathrm{Bin}(K,q_1) + \mathrm{Bin}(N-K,q_0) = k)$, where $q_0$ and $q_1$ are parameters in $[0,1]$\;
Consider the optimization problem $1-(1-p)^{\sum_{i=1}^{N} a_{i}^{t} s_{i}^{t}} + \lambda \sum_{i=1}^{N} s_{i}^{t}$

\For{each agent $i$}{
    Let $w_i$ be the Whittle index\; 
    \While{Binary Search is not completed}{
        Let $m_i$ be the current estimation for the Whittle index \;
        Perform Q-iteration with the following update: 
        \begin{equation}
            Q(s_{i}^{t},a_{i}^{t} = -m_i*a_{i}^{t} + \frac{1-(1-p)^{K}}{T^{t}} + \lambda s_{i}^{t} + \gamma \sum_{s_{i}^{t+1}} \sum_{T^{t+1}} P(s_{i}^{t+1} | s_{i}^{t}, a_{i}^{t})*p(T^{t+1})*V(s_{i}^{t+1},T^{t+1})
        \end{equation}
        Compute the $Q$ values for $Q^{m_i}(s_{i}^{t},T^{t},0)$, $Q^{m_i}(s_{i}^{t},T^{t},1)$ \; 
        
        If $Q^{m_i}(s_{i}^{t},T^{t},0) > Q^{m_i}(s_{i}^{t},T^{t},1)$, then decrease $m_i$\;
        Otherwise, increase $m_i$
    }
    Let $w_i$ be the resulting value for $m_i$
}
Pick the arms with the $K$ highest values for $w_i$

 \caption{Sufficient Whittle-Index for Matching + Activity}
\end{algorithm}

\begin{algorithm}[H]
\SetAlgoLined
\KwResult{Find optimal actions through a combo of Whittle + Greedy}
Consider $N$ agents to be in state $s_{i}^{(t)}$ at time $t$\; 
Let each agent have a probability of matching, $p_{i}$\;
Additionally, let each agent be in one of $G$ groups, with agent $i$ being in group $g_i$\; 
Let the transition probabilities for group $g$ be denoted $T_{g}$, and therefore, the transition probabilities for agent $i$ be denoted $T_{g_{i}}$\;
We select $K$ agents to notify at timestep $t$, so to maximize the $\gamma$-discounted reward (see Section 4)\;
Objective: $\mathbb{E} _{(\mathbf{s},\mathbf{a})\sim (\mathcal{P},\pi)} \sum_{t=1}^{\infty} \gamma^{t} (R_{G}(\{s_{1}^{(t)} \cdots s_{N}^{(t)}\},\{a_{1}^{(t)} \cdots a_{N}^{(t)}\}) + \lambda  [\sum_{i=1}^{N} R_{i}(s_{i}^{(t)},a_{i}^{(t)})])$\;
In the matching scenario, $R_{G}(\{s_{1}^{(t)} \cdots s_{N}^{(t)}\},\{a_{1}^{(t)} \cdots a_{N}^{(t)}\} = 1-\prod_{i=1}^{N} (1-p_{i})^{s_{i}^{(t)} a_{i}^{(t)}}$ and $R_{i}(s_{i}^{(t)},a_{i}^{(t)})]) = s_{i}^{(t)}$\;

\For{each agent $i$}{
    Let $w_{i,s_{i}^{(t)}}$ be the Whittle index for agent $i$ in state $s_{i}^{(t)}$ \; 
    Let $x_i = w_i + \frac{p_{i} s_{i}^{(t)}}{1-\gamma}$
}
Pick the arms with the $K$ highest values for $x_i$

 \caption{Whittle + Greedy}
\end{algorithm}

\begin{algorithm}[H]
\SetAlgoLined
\KwResult{Find optimal actions through MCTS}
Consider $N$ agents to be in state $s_{i}^{(t)}$ at time $t$\; 
Let each agent have a probability of matching, $p_{i}$\;
Additionally, let each agent be in one of $G$ groups, with agent $i$ being in group $g_i$\; 
Let the transition probabilities for group $g$ be denoted $T_{g}$, and therefore, the transition probabilities for agent $i$ be denoted $T_{g_{i}}$\;
Let $S$ be an empty set\; 
\texttt{\\}

Consider an MCTS Tree, $M$ rooted at $n_0$\; 
Let the set of children for any node $n$ be denoted $n_{\mathrm{children}}$, the set of ancestors be denoted $n_{\mathrm{ancestors}}$, and the agent corresponding to a node be $n_{\mathrm{agent}}$\;
Let $Q$ be a queue\;
\For{$i \in 1 \cdots N$} {
    Let $n_i$ be a node with depth 1, corresponding to agent $i$\; 
    Add $n_{i}$ to $Q$\;
    Add $n_{i}$ as a child to $n_0$\; 
}
\While{$|Q| > 0$}{
    Let $n_{i}$ be the result of dequeuing $Q$\; 
    Let $d$ be the depth of $n_{i}$\;
    \If{$d<K$}{
        \For{$j \in 1 \cdots N$} {
            \If{$j \neq i \And j \notin \{n_{\mathrm{agent}} | n \in n_{i,\mathrm{ancestors}} \}$}{
                Let $n_{j}$ be a node with depth $d+1$, corresponding to agent $j$\; 
                Add $n_{j}$ to $Q$\;
                Add $n_{j}$ as a child to $n_{i}$\; 
            }            
        }
    }
}

\texttt{\\}
For each node, $n$, consider $v_{n}$ to be the number of times the node was visited, and $r_{n}$ to be the average reward from visiting that node\;
Let $\alpha=\frac{1}{\sqrt{2}}$ be an exploration constant\;

\texttt{\\}
\For{$b \in 1 \cdots K$}{
    Let $\tau=0$
    \While{\tau $\leq \tau_{\mathrm{max}}$}{
        Let $n=n_{0}$\; 
        \While{$\mathrm{depth}(n) < K$} {
            \If{$\exists c$, $c \in n_{\mathrm{children}} \And v_{c}=0$} {
                Let $n=c$\; 
            }
            \Else{
                Let $n$ be the child, $c$, that maximizes $\frac{r_{c}}{v_{c}}  + \alpha * \frac{\sqrt{2*\log{v_{n}}}}{v_{c}}$\;
                Let $n=c$\;
            }
        }
        Let the ancestors of $n$, including $n$, correspond to agents $n_{1} \cdots n_{K-(b-1)}$\;
        Let the Whittle index for agent $i$ be $w_i$\;
        Let the reward be $r=1-\prod_{i=1}^{K-(b-1)}(1-s_{n_i}^{(t)} p_{n_i}) + \sum_{i=1}^{K-(b-1)} w_{i}$\; 
        $v_{n} \rightarrow v_{n}+1$, and repeat for all ancestors\;
        $r_{n} \rightarrow r_{n}+r$, and repeat for all ancestors\; 
        Update $\tau$ with the time passed, in milliseconds, within this loop\;
    }
    Let $n$ be the node with the largest value for $\frac{r_{i}}{v_{i}}$; add $n$ to $S$\; 
    Replace the MCTS root, $n_0$, with the tree rooted at $n$\;
}
\texttt{\\}

Return $S$\;

 \caption{MCTS-based selection}
\end{algorithm}

\begin{algorithm}[H]
\SetAlgoLined
\KwResult{Find optimal actions through MCTS Two Step}
Consider $N$ agents to be in state $s_{i}^{(t)}$ at time $t$\; 
Let each agent have a probability of matching, $p_{i}$\;
Additionally, let $G$ be a map from groups to agents, and $g$ being a map from agents to groups, with agent $i$ being in group $g_i$, and $i \in G_{g_i}$\; 
We consider all agents within a group to have identical transition probabilities\;
Let the transition probabilities for group $g$ be denoted $T_{g}$, and therefore, the transition probabilities for agent $i$ be denoted $T_{g_{i}}$\;
We select $K$ agents to notify at timestep $t$, so to maximize the $\gamma$-discounted reward (see Section 4)\;

\texttt{\\}

Run the Whittle+Greedy algorithm, and retrieve the corresponding agents as $S'_{1} \cdots S'_{K}$\; 

\texttt{\\}
Consider an MCTS Tree, $M$ rooted at $n_0$\; 
Let the set of children for any node $n$ be denoted $n_{\mathrm{children}}$, the set of ancestors be denoted $n_{\mathrm{ancestors}}$, and the agent corresponding to a node be $n_{\mathrm{agent}}$\;
Let $Q$ be a queue\;
\For{$i \in G_{S'_{1}}$} {
    Let $n_i$ be a node with depth 1, corresponding to agent $i$\; 
    Add $n_{i}$ to $Q$\;
    Add $n_{i}$ as a child to $n_0$\; 
}
\While{$|Q| > 0$}{
    Let $n_{i}$ be the result of dequeuing $Q$\; 
    Let $d$ be the depth of $n_{i}$\;
    \If{$d<K$}{
        \For{$j \in G_{S'_{d+1}}$} {
            \If{$j \neq i \And j \notin \{n_{\mathrm{agent}} | n \in n_{i,\mathrm{ancestors}} \}$}{
                Let $n_{j}$ be a node with depth $d+1$, corresponding to agent $j$\; 
                Add $n_{j}$ to $Q$\;
                Add $n_{j}$ as a child to $n_{i}$\; 
            }            
        }
    }
}

Let $S$ be an empty set\;

\For{$b \in 1 \cdots K$}{
    Let $\tau=0$
    \While{\tau $\leq \tau_{\mathrm{max}}$}{
        Let $n=n_{0}$\; 
        \While{$\mathrm{depth}(n) < K$} {
            \If{$\exists c$, $c \in n_{\mathrm{children}} \And v_{c}=0$} {
                Let $n=c$\; 
            }
            \Else{
                Let $n$ be the child, $c$, that maximizes $\frac{r_{c}}{v_{c}}  + \alpha * \frac{\sqrt{2*\log{v_{n}}}}{v_{c}}$\;
                Let $n=c$\;
            }
        }
        Let the ancestors of $n$, including $n$, correspond to agents $n_{1} \cdots n_{K-(b-1)}$\;
        Let the Whittle index for agent $i$ be $w_i$\;
        Let $\bar{s}_{n_i}^{(t)} = T_{g_{i},s_{n_i}^{(t)},1,1}$\;
        Let the reward be $r=1-\prod_{i=1}^{K-(b-1)}(1-\bar{s}_{n_i}^{(t)} p_{n_i}) + \sum_{i=1}^{K-(b-1)} w_{i}$\; 
        Increment $v_{n}$, and repeat for all ancestors\;
        Add $r$ to $r_{n}$, and repeat for all ancestors\; 
        Update $\tau$ with the time passed, in milliseconds, within this loop\;
    }
    Let $n$ be the node with the largest value for $\frac{r_{i}}{v_{i}}$; add $n$ to $S$\; 
    Replace the MCTS root, $n_0$, with the tree rooted at $n$\;
}

 \caption{MCTS Two Step}
\end{algorithm}

\section{Dataset Analysis}

\begin{algorithm}[H]
\SetAlgoLined
\KwResult{Generate 2x2x2 transition matrices, $T_1, T_2 \cdots T_d$ for $d$ agents}
Let $N$ be the number of volunteers\;
Let $r_i$ denote the number of weeks served by volunteer $i$\;
Let $v^{(i)}_{j}$ denote whether volunteer $i$ serves \textbf{their} $\mathrm{j^{th}}$ week 
Let $T_{d}$ be the transition matrix indexed by $s,a,s^\prime \in \{0,1\}$\;
Finally, let $V_d = \{v^{(i)}|r_i=d\}$ denote the set of volunteers that served $d$ days\;
\begin{equation}
    T_{d,s,a,s^\prime} = \frac{\sum_{v^{(i)} \in V_d} \sum_{j=1}^{r_i-2} \mathbbm{1}[v^{(i)}_{j}=s \wedge v^{(i)}_{j+1}=a \wedge v^{(i)}_{j+2}=s^\prime]}    {\sum_{v^{(i)} \in V_d} \sum_{j=1}^{r_i-2} \mathbbm{1}[v^{(i)}_{j}=s \wedge v^{(i)}_{j+1}=a]}
\end{equation}

 \caption{Generating Transition Function}
\end{algorithm}

\section{Problem Variants for Food Rescue}
We tackle several variants of the matching + activity problem motivated by real-world challenges in the food rescue context. 
Each problem involves a variation on the Whittle index algorithm and problem formulation to account for real-world complications. 

% \subsection{Volunteer Preferences}
% Volunteers are heterogeneous, with different preferences for different food rescue trips. 
% For example, volunteers might prefer to service trips closer to their home, or to service shorter trips. 
% To capture such an idea, we consider each volunteer to have a rating for a trip, which we denote $r_{i}^{t} \in [0,1]$. 
% We solve the matching problem under the linearity assumption, and show that incorporating preferences can still be solved through a Whittle index. 
% Maximizing the number of matches then becomes solving the following question: 
% \begin{equation}
%     \sum_{t=1}^{T} \sum_{i=1}^{N} p_{i}^{t} s_{i}^{t} a_{i}^{t}
% \end{equation}
% Such a problem can still be written under the Whittle index framework, because the reward, $R(s_{i}^{t},a_{i}^{t}) = p_{i}^{t} s_{i}^{t} a_{i}^{t}$, and is therefore separable. 
% At each timestep, we re-solve for the value of the subsidy using a Q-learning framework, where the Q-value for state $s_{i}^{t}$ and action $a_{i}^{t}$ under subsidy $m$ is 
% \begin{equation}
%     Q(s_{i}^{t},a_{i}^{t}) = -m*a + p_{i}^{t} s_{i}^{t} a_{i}^{t} + \gamma \sum_{s' \in S} V(s') P_{i}(s_{i}^{t},a_{i}^{t},s') 
% \end{equation}
% Running Q iteration and finding an $m$ so $Q(s_{i}^{t},1) = Q(s_{i}^{t},0)$ solves the Whittle index and allows us to incorporate preferences. 

\subsection{Variable K}
In a food rescue context, the parameter $K$ might not be known a priori, or it might be the scenario that organizers can notify as many volunteers as needed, though they might incur some implicit penalty, such as burnout, from notifying too many volunteers. 
We show that the fixed K scenario can be solved through Q-learning without a need for a Whittle index, as each arm can be solved separately. 
In essence, each arm (volunteer), $i$, can be viewed as a decision problem of whether or not to notify volunteer $i$. 
The reward for pulling arm $i$ is $a_{i}^{t} s_{i}^{t}$, however, we note that burnout states (which we cover in Section INSERT SECTION) makes it so it's not always optimal to pull all arms. 
Because of the independence of the arms, we solve each arm through Q-learning, using the following Q function
\begin{equation}
    Q(s_{i}^{t},a_{i}^{t}) = s_{i}^{t} a_{i}^{t} + \gamma \sum_{s' \in S} V(s') P_{i}(s_{i}^{t},a_{i}^{t},s') 
\end{equation}
We then select the higher of $Q(s_{i}^{t},0)$ and $Q(s_{i}^{t},1)$ for each arm and pull accordingly, with no need to solve for Whittle subsidies.

\section{Metrics}
\begin{algorithm}[H]
\SetAlgoNlRelativeSize{0}
\SetNlSty{textbf}{(}{)}
\KwResult{Compute active rate, $r_{a}$, and match rate, $r_{m}$}

Initialize active rates, $r_{a}=0$, and match rates, $r_{m} = 0$ \;
Let the match probability be $p$\;

\For{episode $t = 1, 2, \ldots, E$}{
Perform action $\mathbf{a_{i}^{(t)}}$,

Let $r_{a} \rightarrow r_{a} + \frac{1}{N} \sum_{i=1}^{N} R(s_{i}^{(t)})$; this computes the fraction of active volunteers\;

Let $r_{m} \rightarrow r_{m} + 1-(1-p)^{\sum_{i=1}^{n} (1-a_{i}^{(t)}) \mathbbm{1}[s_{i}^{(t)}]}$; this measures the probability that all notified volunteers plus active volunteers reject the trip\;

Update $s_{i}^{t+1} ~ P_{i}(s_{i}^{(t)}, a_{i}^{(t)}, s_{i}^{t+1})$ for each arm $i$

}

Return $\frac{r_{a}}{T}$ and $\frac{r_{m}}{T}$\;

\caption{Metrics during Volunteer Matching}
\end{algorithm}

\section{Heuristic Details}
\begin{algorithm}[H]
\SetAlgoNlRelativeSize{0}
\SetNlSty{textbf}{(}{)}
\KwResult{Select actions that maximize matches}
Let the match probability be $p$\;
Let $N_i(s,a,s^\prime)$ be the counter for number of transitions from $s \rightarrow a \rightarrow s^\prime$ for volunteer $i$ \; 

\For{episode $t = 1, 2, \ldots, E$}{
Compute an estimated transition matrix
\begin{equation} 
\hat{P_i}_{s,a,s^\prime} = \frac{V_i(s,a,s^\prime)}{V_i(s,a,s^\prime) + V_i(s,a,1-s^\prime)}
\end{equation}
Suppose we play the intervene action; what proportion will volunteer $i$ be active? \; 
Using $\hat{P_i}$, compute the stationary distribution, $\mu_i$ using the eigenvectors of $\bar{P}_{i}$, which reduces $P_i$ to two states, $D=0$ and $E=1$ \; 
Let $a_{i}^{t} = 1$ for the arms with the $K$ highest values of $\mu_{i,1}$, and let $a_{i}^{t}=0$ otherwise \; 
Increment $V_i(s,a,s^\prime)$ based on observed state transitions;
}

\caption{Optimizing Matches}
\end{algorithm}

\section{More Theory}
\subsection{Optimality of Matching Algorithm}
We will prove that our matching algorithm, with known transitions, is asymptotically optimal, and achieves $\mathcal{O}(1)$ regret. 
The task is to find a policy, $\pi: \mathcal{S}^{N} \rightarrow \mathcal{A}^{N}$, which maps the state of each arm, to the actions for each arm. 
We will prove the following theorem: 
\begin{theorem}
    Let $P_i$ be the transition probabilities for each arm, where $P_i(s,a,s^\prime)$ indicates the probability of going from state $s$ to state $s^\prime$ when taking action $a$. Let the matching probability for a given arm be $p$, and let each arm be in state $s_{i}^t$. Consider the presence of two sets of states, $D$ and $E$. Our goal is to find actions, $a_{i}^t$ so that the following is maximized
    \begin{equation}
        R_{G}(\{s_{1}^{(t)} \cdots s_{N}^{(t)} \},\{a_{1}^{(t)} \cdots a_{N}^{(t)}\}) =  1-\prod_{i=1}^{N}(1-p_{i})^{(1-a_{i}^{(t)})\mathbbm{1}[s_{i}^{(t)} \notin E]}
    \end{equation}

    Let $\bar{P_i} = P_i(s,1,s^\prime)$ be the Markov chain corresponding to pulling arm $i$. We view $\bar{P_i}$ as a two-state Markov chain, reducing the sets of states $D$ and $E$ to singleton states $D=0$ and $E=1$. Assume that this Markov chain is ergodic, then let the steady state when repeatedly taking action $a_{i}$ be $\bar{P_i}\mu_i^{a_i}=\bar{P_i}$. Assume that $\bar{P}_i(0,1,1) > \bar{P}(0,0,1) \forall i$; that is, intervening assists in getting to state 1. If we let $M_i = \mu_{i,1}^{a_i} \bar{P}_i(1,1,1) + (1-\mu_{i,1}) \bar{P}_i(0,1,1) = \mu_{i,1}^{a_i}$ be the matching index, then let $\pi$ be the policy that pulls the $K$ arms corresponding to the largest values of $M_i$. Then $\pi$ is asymptotically optimal and achieves $\mathcal{O}(1)$ regret. 
\end{theorem}

We start by introducing several facts of Markov chains

\begin{lemma}
    The Markov Chain representing states for arm $i$ mixes in $\mathcal{O}(\mathrm{log}(\frac{1}{\epsilon}))$ for a fixed arm transition matrix, $P_i$. 
\end{lemma}
\begin{proof}
    Note that, using $\bar{P}_i$, we can view the transition of arm $i$ as a two-state Markov chain. 
    From Theorem (INSERT NUMBER) in INSERT REFERENCE, we note that the mixing time for a Markov chain, $t_{\mathrm{mix}}(\epsilon) \leq \mathrm{log}(\frac{1}{\epsilon \mu_{\mathrm{min}}}) \frac{1}{\lambda_2}$, where $\lambda_2$ is the second eigenvalue of $\bar{P}_i$. For a fixed $P$, this is $\mathcal{O}(\mathrm{log}(\frac{1}{\epsilon}))$
\end{proof}

\begin{lemma}
    Once a Markov chain is well mixed, the optimal policy, $\pi^*$ is independent of $t$ and can be represented as a distribution. 
\end{lemma}
\begin{proof}
    Suppose that the distribution for arm $i$ increases by $\epsilon$ from time step $t$ to $t+1$, and similarly, that arm $j$ decreases by $\epsilon$ from time step $t$ to $t+1$. At time step $t$, it was optimal to pull arm $j$ with some probability $b_{j}^{t}$. That is, at time step $t$, the minimizing solution to 
    \begin{equation}
        \sum_{i=1}^{N} (1-a_{i,t}) \Pr[s_{i}^{t} \notin E]
    \end{equation}
    is to pull arm $j$ with some probability $b_{j}^{t}$.
    By moving $\epsilon$ away from arm $j$, it must be the case that doing so increases $\Pr[s_{i}^{t+1} \notin E]$ more than it decreases $\Pr[s_{j}^{t+1} \notin E]$. 
    However, note that for a well mixed Markov chain, it must be the case that state probabilities are the same between states; therefore, applying $b_{i}^{t+1},b_{j}^{t+1}$ would result in the same performance gain. 
    Therefore, $b_{i}^{t}=b_{i}^{t+1}, b_{j}^{t}=b_{j}^{t+1}$, so $b$ is constant across timesteps after well mixing. 
\end{proof}

\begin{lemma}
    For a well mixed Markov chain, there always exists a $\pi^*$ that is deterministic (a pure strategy essentially). 
\end{lemma}
\begin{proof}
    By Lemma (LEMMA NUMBER), we know that the optimal policy, $\pi^*$ can be represented as sampling from some distribution. Let $b_{i}^{t} = \Pr[a_{i}^{t}=1]$; note that this is general.  
    We can view the whole Markov chain, both with $a_{i}^{t} = 0$ and $a_{i}^{t}$, as a 2-state markov chain, with steady state $\nu_i$, which solves 
    \begin{equation}
        \nu_i \begin{bmatrix}
        b_{i}^{t} \bar{P_i}(0,1,0) + (1-b_{i}^{t})\bar{P_i}(0,0,0) & b_{i}^{t} \bar{P_i}(0,1,1) + (1-b_{i}^{t})\bar{P_i}(0,0,1) \\
        b_{i}^{t} \bar{P_i}(1,1,0) + (1-b_{i}^{t})\bar{P_i}(1,0,0) & b_{i}^{t} \bar{P_i}(1,1,1) + (1-b_{i}^{t})\bar{P_i}(1,0,1) \\
        \end{bmatrix}
        = \nu_i 
    \end{equation}
Note that, because $\nu_i$ is a steady state vector, $\nu_{i,0} = 1-\nu_{i,1}$
    Therefore, by solving the matrix equation, we get 
    \begin{equation}
        \nu_{i,1} = \frac{b_{i}^{t}(\bar{P_i}(0,1,1)-\bar{P_i}(0,0,1))+\bar{P_i}(0,0,1)}{b_{i}^{t}(\bar{P_i}(0,1,1)+\bar{P_i}(1,0,1)-\bar{P_i}(1,1,1)-\bar{P_i}(0,0,1)) + \bar{P_i}(0,0,1)-\bar{P_i}(1,0,1)+1}
    \end{equation}
    and note that the critical points exist only if $\bar{P_i}(0,1,1) = \bar{P_i}(0,0,1)$. 
    But by the assumption, we note that $\bar{P_i}(0,1,1) > \bar{P_i}(0,0,1)$, and therefore, all extrema are on the endpoints, which corresponds to all $b_{i}^{t} \in \{0,1\}$. 
    Note that such an argument naturally extends across all $a_{i}^{t} \forall i$ when taking gradients, as critical points require that each dimension has derivative 0, which does not exist. 
    Therefore, optimal policies, $\pi*$, require that all $b_{i}^{t} \in \{0,1\}$, meaning that all policies are deterministic. 
\end{proof}

We combine these lemmas to prove the optimality of our matching algorithm
\begin{proof}
We note that by Lemma (LEMMA NUMBER), that the optimal policy $\pi^*$ must pull on exactly $K$ arms for each timestep, with the same arm being pulled in each timestep, as there are no interior optima. 
Recall that we aim to maximize 
\begin{equation}
    \sum_{t=1}^{T} 1-(1-p)^{\sum_{i=1}^{N} (1-a_{i}^{t})\mathbbm{1}[s_{i}^{(t)} \notin E]}
\end{equation}
This is the same as minimizing $\sum_{i=1}^{N} (1-a_{i}^{t})\mathbbm{1}[s_{i}^{(t)} \notin E]$, subject to $\sum_{i=1}^{N} a_{i}^{t} \leq K$. 
We remove the dependence on $t$ due to homogeneity across time steps, and note that increasing $a_{i}$ can only decrease the sum, leading to minimizing $\sum_{i=1}^{N} (1-a_{i})\mathbbm{1}[s_{i} \notin E], \sum_{i=1}^{N} a_{i} = K$. 
Because the Markov chain is well mixed (by assumption), and that $\pi*$ is deterministic, we note that when $a_i=1$, $\Pr[s_{i} \notin E] = \mu_{i,1}^{1}*\bar{P}_i(1,1,1) + \mu_{i,0}^{1}*\bar{P}_i(0,1,1)$
\nrcomment{Is this the same as mu i,1 when it's well mixed? I think so, but not 100\% sure}
For well mixed Markov chains, this is the same as $\mu_{i,1}$. 
Therefore, minimizing $\mathbb{E}[\sum_{i=1}^{N} (1-a_{i}^{t})\mathbbm{1}[s_{i}^{(t)} \notin E]] = \sum_{i=1}^{N} (1-a_{i})\Pr[s_{i} \notin E] = \sum_{i=1}^{N} (1-a_{i}) \mu_{i,1}$. 
Minimizing this sets $a_{i}=1$ for the largest values of $\mu_{i,1}$.
Note that, after mixing, this algorithm achieves 0 regret in expectation, and that mixing occurs in (X) time, which is constant in the number of total time steps, $T$. 
Additionally, note that our Markov chain is represented as a 2 state, 2 action chain, meaning tha the mixing time is $\mathcal{O}(1)$. 
\nrcomment{Can you even use regret with an oracle algorithm? Check terminology}

\end{proof}
